# Supplementary material for: Production and characterization of a fragmented spinor Bose-Einstein condensate
Source: arXiv:2010.15739 ancillary file (2020-10-29)
Supplement: Supplementary file 1 [file Supplemental.pdf]

# Production and characterization of a fragmented spinor Bose-Einstein condensate

Bertrand Evrard, An Qu, Jean Dalibard, and Fabrice Gerbier
(Dated: July 11, 2020)

## I. GROUND STATE

In this section we recall theoretical results regarding the ground state of the Hamiltonian of a gas of bosonic spin-1 atoms in the single-mode approximation [1]

$$\hat{H} = -q\hat{N}_0 + \frac{U_s}{2N}\hat{\boldsymbol{S}}^2 , \tag{1}$$

where $q$ is the quadratic Zeeman energy and $U_s$ the spin-spin interaction energy. The total spin $\hat{\boldsymbol{S}}^2$ can be written

$$\begin{aligned}\hat{\boldsymbol{S}}^2 = \hat{S}_z^2 + N + \hat{N}_0 + 2\hat{N}_0(N-\hat{N}_0)\\ +2(\hat{a}_0^{\dagger 2}\hat{a}_{+1}\hat{a}_{-1} + \hat{a}_0^2\hat{a}_{+1}^\dagger\hat{a}_{-1}^\dagger) .\end{aligned} \tag{2}$$

### A. Bogoliubov Approximation

In the small depletion regime $N - N_0 \ll N$, the Bogoliubov approximation leads to the quadratic Hamiltonian

$$\hat{H}_B = (q+U_s)\left(\hat{N}_{+1}+\hat{N}_{-1}\right) + U_s\left(\hat{a}_{+1}\hat{a}_{-1} + \hat{a}_{+1}^\dagger\hat{a}_{-1}^\dagger\right) , \tag{3}$$

up to terms of order $1/N$ and an additive constant. Using the Bogoliubov transformation

$$\hat{\alpha} = \cosh(\theta)\hat{a}_{+1} - \sinh(\theta)\hat{a}_{-1}^\dagger , \tag{4}$$

$$\hat{\beta} = \sinh(\theta)\hat{a}_{+1}^\dagger - \cosh(\theta)\hat{a}_{-1} , \tag{5}$$

with $\tanh(2\theta) = -U_s/(q+U_s)$, the Hamiltonian (3) can be written in the diagonal form $\hat{H}_B = \hbar\omega_B(\hat{\alpha}^\dagger\hat{\alpha} + \hat{\beta}^\dagger\hat{\beta})$, with the Bogoliubov energy $\hbar\omega_B = \sqrt{q(q+2U_s)}$.

The longitudinal spin is $\hat{S}_z = \hat{N}_{+1} - \hat{N}_{-1} = \hat{\alpha}^\dagger\hat{\alpha} - \hat{\beta}^\dagger\hat{\beta}$. The conservation of $\hat{S}_z$ implies that Bogoliubov excitations are always created by pairs, one in each mode $\alpha, \beta$. Taking this constraint into account, the energy splitting between the ground state and the first exited state is $\Delta E = 2\hbar\omega_B$.

For $q \ll U_s$, we can compute the mean value of some observables of interest in the ground state of the Hamiltonian $\hat{H}_B$:

$$\langle N_{\pm 1}\rangle_B \simeq \sqrt{\frac{U_s}{8q}} , \tag{6}$$

$$\Delta N_{\pm 1 B}^2 = \langle N_{\pm 1}\rangle_B \,(1 + \langle N_{\pm 1}\rangle_B) , \tag{7}$$

$$\langle \hat{\boldsymbol{S}}^2\rangle_B \simeq \frac{2Nq - U_s}{\hbar\omega_B} . \tag{8}$$

Note that the value of $\langle\hat{\boldsymbol{S}}^2\rangle_B$ is reduced significantly below the shot-noise value $2N$ for $q \sim U_s/N$, while the depletion of $m=0$, $\langle N_{+1} + N_{-1}\rangle_B$ becomes macroscopic only for $q \sim U_s/N^2$. This can be understood as an effect of bosonic amplification: atoms involved in singlet pairs have a larger probability to be measured in $m=0$ as long as this state remains the only macroscopically populated one.

### B. Ground state at $q = 0$

When the magnetic field vanishes, the eigenstates of the Hamiltonian (1) are the collective spin states [1–3]

$$|N,S,M\rangle = \frac{1}{\sqrt{\mathcal{N}}}\,\hat{S}_-^P\,\hat{a}_{+1}^{\dagger S}\,\hat{A}^{\dagger Q}\,|\text{vac}\rangle , \tag{9}$$

where $P = S - M$, $2Q = N - S$. We introduced the spin lowering operator $\hat{S}_- = \sqrt{2}(\hat{a}_{-1}^\dagger\hat{a}_0 + \hat{a}_0^\dagger\hat{a}_{+1})$ and the singlet pair creation operator $\hat{A}^\dagger = \hat{a}_0^{\dagger 2} - 2\hat{a}_{-1}^\dagger\hat{a}_{+1}^\dagger$. Finally the normalization constant is

$$\mathcal{N} = \frac{S!(N-S)!!(N+S+1)!!(S-M_z)!(2S)!}{(2S+1)!!(S+M_z)!} . \tag{10}$$

For $M = 0$ and $N$ even, the ground state is the collective spin singlet

$$|N,0,0\rangle = \frac{1}{\sqrt{(N+1)!}}\hat{A}^{\dagger N/2}|\text{vac}\rangle . \tag{11}$$

This states verifies

$$\langle N,0,0|\hat{\boldsymbol{S}}^2|N,0,0\rangle = 0 , \tag{12}$$

$$\langle N,0,0|\hat{N}_0|N,0,0\rangle = \frac{N}{3} . \tag{13}$$

For $M = 0$ and $N$ odd, a simple algebraic manipulation of (9) shows that the ground state is obtained either by adding to a particle in $m = 0$ to the $(N-1)$ singlet state, or by removing a particle in $m = 0$ from the $(N+1)$ singlet state

$$|N,1,0\rangle = \frac{\sqrt{3}}{\sqrt{N+2}}\,\hat{a}_0^\dagger\,|N-1,0,0\rangle \tag{14}$$

$$= \frac{\sqrt{3}}{\sqrt{N+1}}\,\hat{a}_0\,|N+1,0,0\rangle . \tag{15}$$

This states verifies

$$\langle N,1,0|\hat{\boldsymbol{S}}^2|N,1,0\rangle = 2 , \tag{16}$$

$$\langle N,1,0|\hat{N}_0|N,1,0\rangle = \frac{3N+2}{5} . \tag{17}$$

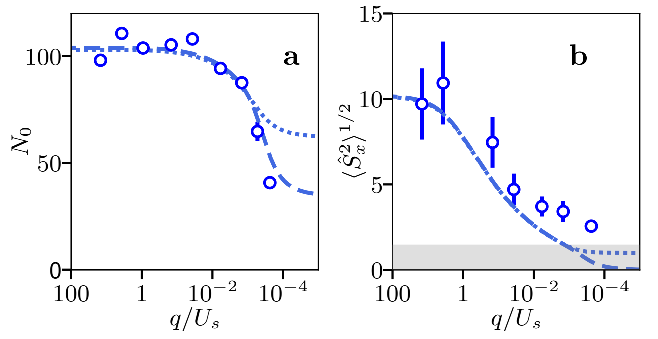


FIG. 1. Evolution of $\langle \hat{N}_0 \rangle$ (**a**) and $\sqrt{\langle \hat{S}_x^2 \rangle}$ (**b**) versus $q$ in the ground state of the Hamiltonian (1) for $S_z = 0$ and $N$ even (dashed line) or odd (dotted line). The blue dots correspond to the experimental data. For these data, the parity of $N$ was unknown and presumably fluctuating. The discrepancy between experimental data and the predictions of this simplified theoretical model is discussed in § II B.

Note the dramatic change of the mean value of $\hat{N}_0$, from $N/3$ when $N$ is even [Eq. (13)] to $\simeq 3N/5$ for $N$ odd [Eq. (17)]. We can reformulate this result in the following way: starting from the singlet state with $N+1$ (even) particles, one measures the spin along $z$ of a first particle. Because of the symmetry of the singlet state, the three possible results $m = 0, \pm 1$ have equal probabilities 1/3. Now, if the particle is detected in $m = 0$, the state of the $N$ remaining particles is given by Eq. (15). The probability for detecting a second particle again in $m = 0$ is not anymore $\approx 1/3$, but has increased to $\approx 3/5$. This counterintuitive result signals the highly non-classical nature of the $N$-particle singlet state, and it is reminiscent of the way the relative phase between two independent condensates builds up in a succession of individual measurements [4, 5].

### C. Numerical diagonalization

We show in figure 1 our predictions for the evolution of $\langle \hat{N}_0 \rangle$ and $\sqrt{\langle \hat{S}_x^2 \rangle}$ during the ramp on $q(t)$. These results were calculated using the instantaneous ground state, obtained from a numerical diagonalization of the Hamiltonian (1), assuming $S_z = 0$. For comparison, we also show our experimental results for the evolution of these observables.

## II. SIMULATION OF THE EXPERIMENTAL SEQUENCE

### A. Adiabatic ramp in an ideal situation

We show in Fig. 2 the results of a numerical calculation of the state $|\psi(t)\rangle$ during the ramp. We compare at various times the values of $n_0 = N_0/N$ and

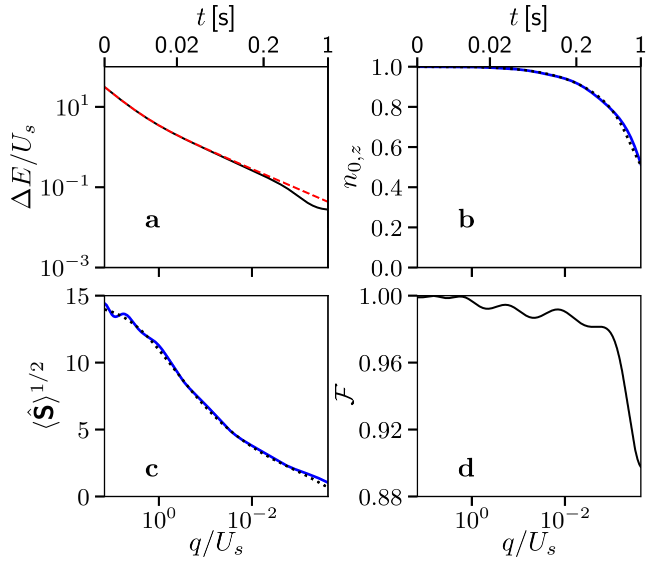


FIG. 2. **a.** Energy gap between the ground state $|\mathrm{GS}(B)\rangle$ and the first excited state. The solid line is the result of numerical diagonalization, the dashed line corresponds to Bogoliubov approximation. **b,c.** Continuous blue lines: evolution of $n_0$ (**b**), and of the total spin (**c**) over the ramp, calculated for the solution of the Schrödinger equation $|\psi(t)\rangle$. The dotted lines correspond to the expectation values for the instantaneous ground state $|\mathrm{GS}[B(t)]\rangle$. **d.** Fidelity between the solution of the Schrödinger equation and the instantaneous ground state $\mathcal{F}(t)$ over the ramp. In this simulation, $N$ is chosen even ($N = 104$). The deviation to adiabaticity is smaller for $N$ odd.

$\sqrt{\langle \hat{\mathbf{S}}^2 \rangle}$ with the expectation values for the instantaneous ground state $|\mathrm{GS}[B(t)]\rangle$. We see only little deviations, indicating that the adiabaticity criterion is well verified. This is confirmed by looking at the evolution of the overlap of $|\psi(t_f)\rangle$ with the instantaneous ground state, $\mathcal{F}(t) = |\langle \mathrm{GS}[B(t)]|\psi(t)\rangle|^2$. At the end of the ramp, for $N = 104$ (even), we compute $\mathcal{F}(t_f) = 0.90$, and the overlap with the ground state at $B = 0$ (*i.e.*, the singlet $S = 0$) is $|\langle \mathrm{GS}(0)|\psi(t_f)\rangle|^2 = 0.82$. For $N = 103$ (odd), the overlaps with the ground state at $B = B_f$ or with the ground state at $B = 0$ (*i.e.*, $S = 1$) are both $> 0.99$.

### B. Decoherence during the adiabatic ramp

Our characterization of the state at the end of the ramp reveals significant discrepancies with the simple theory presented above, as shown in the figure 1 of this Supplementary Material. We measured a smaller $N_0$ and a larger spin length, especially in the $xy$ plane. In addition, the reconstructed many-body state (see § V B) has a (small) non-zero entropy, whereas the fully deterministic evolution discussed above should lead to a pure state. In this subsection, we discuss two possible sources of decoherence which when combined, can explain quantitatively

our results.

A first source of decoherence originates from the collisions between atoms of the condensate and particles of the residual gas filling the science chamber. These collisions result in one-body losses, occurring at a rate $1/\tau$ independent on the Zeeman state $m$ of the atoms. Thus, during the time interval $\mathrm{d}t \ll \tau$, an atom in state $m$ is lost with a probability $\mathrm{d}p_m = \langle \hat{N}_m(t)\rangle\, \mathrm{d}t/\tau$.

We incorporated this process in the numerical simulation of the adiabatic ramp using a quantum trajectory approach [6–8]. At each time step of the algorithm, we draw a random number $\epsilon \in [0,1]$. If $\epsilon > \sum \mathrm{d}p_m$, no atom is lost and the state evolves under the regular Hamiltonian (1) for the atom number $N(t)$ [9]. If $\epsilon < \sum \mathrm{d}p_m$, an atom is lost and we draw another random number to decide the Zeeman state $m$ of this atom. We then apply the jump operator $\hat{a}_m$ to the state, and continue with the Hamiltonian evolution. We repeat this simulation either a hundred times to extract one or two body observables or a thousand times to reconstruct the density matrix, and we look at averaged quantities. The $1/e$ lifetime of our samples is $\simeq 76\,$s which corresponds to $\simeq 1.4$ atoms lost on average over the ramp. By including this loss rate in the numerical simulation of the ramp, we obtained an improved agreement with the data, but the deviations discussed at the beginning of this paragraph still remain significant, pointing towards the presence of an additional decoherence mechanism.

We added therefore another stochastic element to the evolution of our system, corresponding to a "spin-flip", *i.e.* a random change of the Zeeman state of an atom of the fragmented BEC. As for one-body losses, we incorporate this process in the numerical simulation following the quantum trajectory approach. There are now nine jump operators

$$\hat{C}_{m,m'} = \sqrt{k_f}\; \hat{a}^\dagger_{m'} \hat{a}_m\,, \tag{18}$$

with $m, m'$ indicating the initial and final Zeeman states, and $k_f$ is the flip rate. This rate is assumed to be the same for all couples $(m, m')$, so that this additional relaxation process is isotropic.

We show in figure 3 the values of typical observables at the end of the ramp, versus the mean number of spin flips. For this figure, the one-body loss described above is also taken into account, assuming that 1.4 atoms are lost on average during the ramp. We observe an overall very good agreement between the experimental results and the predictions of the simulation for a number of flips during the ramp $N_{\mathrm{flip}} \simeq 2.8$. For this particular value, the simulated density matrix is very similar to the one obtained by the MaxLik reconstruction (see § V B), as shown in figure 4.

While spin-flips appear as possible candidates to model decoherence in our system, the underlying microscopic mechanism remains to be investigated in detail. A possible line of approach could start from the Bogoliubov Hamiltonian for a spinor gas (see e.g. § 5.1 in [1]), which for a uniform system involves terms as $\hat{a}^\dagger_{0,m'_1}\hat{a}_{0,m_1}\hat{a}^\dagger_{\boldsymbol{k},m'_2}\hat{a}_{\boldsymbol{k},m_2}$, where the wave vector $\boldsymbol{k}$ is nonzero. Treating the set of uncondensed ($\boldsymbol{k} \neq 0$) particles as a reservoir, one can write a master equation for the condensate $\boldsymbol{k} = 0$ (see e.g. [10] for an approach of this type for a scalar condensate). In this equation, the jump operators will have a structure similar to Eq. (18). Note that further work is still needed to adapt precisely this scheme to the case of a trapped condensate described in the single mode approximation.

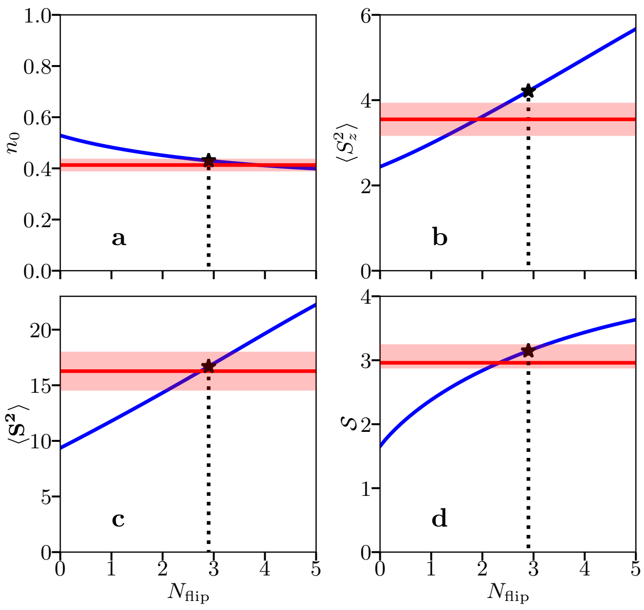


FIG. 3. Results from the quantum trajectory analysis. The blue lines show the mean values of typical observables at the end of the adiabatic ramp versus the average number of spin flips. This simulation also takes into account one-body losses, with a rate determined experimentally and corresponding to an average number of lost atoms $N_{\mathrm{lost}} = 1.4$. For the measurement of the spin (**b** and **c**), we also added the contribution of the detection noise (see § III). We performed these simulations for odd and even initial atom numbers ($N_{\mathrm{i}} = 103$ and 104) and we show here the averaged results. The red lines show the outcomes of direct measurements (**a**,**b**,**c**), or of the reconstructed MaxLik state for the entropy (**d**) (see § V B). The pink area corresponds to two standard errors in **a**,**b** and **c** and to the 68% confidence interval for **d**. The black dotted line indicates the optimal number of flips $N_{\mathrm{flip}} \simeq 2.8$.

## III. NOISE DECONVOLUTION

The contribution of the detection noise in the measurements of $S_z$ (possibly after a spin rotation of the state) is not negligible. We describe here the procedure to remove this contribution in order to evaluate the spin squeezing (see main text) and for the MaxEnt reconstruction (§ V C below). The dominant contribution to the detection noise comes from the shot noise on stray light and

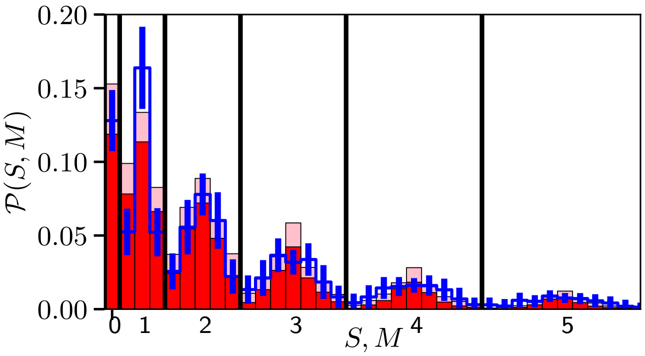


FIG. 4. Blue line: density matrix obtained from the quantum trajectory simulation for $N_{\rm loss} = 1.4$ and $N_{\rm flip} = 2.8$ (blue line). Red bars: density matrix obtained from the MaxLik reconstruction (the pink area indicates the confidence interval). We only show the diagonal elements in the $S, M$ basis (both states are almost diagonal in this basis). The solid lines delimit the subspaces of total spin $S$. Within a subspace, the states are ordered by increasing $M_z$ from $-S$ to $+S$ (the labels refer to the value of $S$).

it is normally distributed [11]

$$\mathcal{P}_{\rm noise}(x) = \frac{1}{\sqrt{2\pi\sigma_{\rm noise}^2}} e^{-x^2/2\sigma_{\rm noise}^2}\,, \tag{19}$$

with a standard deviation $\sigma_{\rm noise} \simeq 2.3$ atoms for the measurements of $S_z$. Let $\rho^R$ be the state of the system after a spin rotation. The probability of the outcome $S_z^{\rm (meas)}$ in a measurement of $\hat{S}_z$ is

$$\mathcal{P}\left(S_z^{\rm (meas)}|\rho^R\right) = \sum_{|M|\leq N} \mathcal{P}_{\rm noise}(S_z^{\rm (meas)} - M)\, \mathcal{P}(M|\rho^R)\,, \tag{20}$$

with

$$\mathcal{P}(M|\rho^R) = \sum_{S\geq |M|} \langle S, M|\rho^R|S, M\rangle\,, \tag{21}$$

the distribution of $S_z$ for the state $\rho^R$. In practice, we fit to the measured distribution of $S_z$ the expression (20), with each probability $\mathcal{P}(M|\rho^R)$ ($M = -N, -N+1, \ldots, N$) as a free parameter. This procedure gives access to the "real" distribution $\mathcal{P}(M|\rho^R)$, and in particular to its second moment. In the absence of rotation (resp. for $\pi/2$ rotation around $y$), this yields the expectation value $\langle \hat{S}_z^2\rangle$ (resp. $\langle \hat{S}_x^2\rangle$) for the state $\rho$ before rotation. The results are given in table I.

## IV. SINGLE PARTICLE DENSITY MATRIX

The single particle density matrix is defined by

$$\rho_{j,k}^{(1)} = \frac{1}{N}\langle \hat{a}_j^\dagger \hat{a}_k\rangle\,, \tag{22}$$

| | $\langle \hat{S}_z^2\rangle$ | $\langle \hat{S}_x^2\rangle$ |
|---|---|---|
| Measured | $3.55 \pm 0.36$ | $6.36 \pm 0.70$ |
| Inferred | $1.17 \pm 0.36$ | $4.37 \pm 0.64$ |

TABLE I. Results of the noise removal for the observables $\hat{S}_z^2$ and $\hat{S}_x^2$.

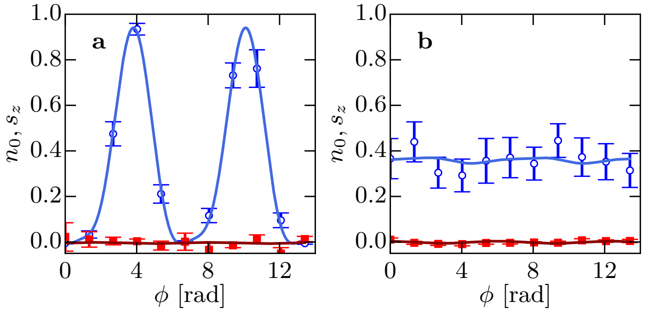


FIG. 5. Evolution of the reduced population $n_0$ (blue dots) and of the spin $s_z$ (red squares) under the rotations $\mathcal{R}_y(\frac{\pi}{4})\mathcal{R}_z(\phi)$ for a polar state (**a**) and a fragmented state (**b**). The solid lines are the fits to the experimental data from which we extract $\rho^{(1)}$.

where $j, k \in \{0, \pm 1\}$. It can be fully determined by looking at the evolution of the state under a composition of two rotations. First, we rotate the state around the $z$-axis by a variable angle $\phi$. Then, we rotate the state around the $y$-axis by an angle $\pi/4$. We measure $N_0^R(\phi)$ and $S_z^R(\phi)$. Since the duration of the rotation $\sim 10\,\mu$s is much shorter than $\hbar/U_s$ and $\hbar/q$, we can neglect the effect of interactions and of the Zeeman shift during this time interval and we get

$$\begin{aligned} N_0^R(\phi) =& \frac{N+N_0}{4} + \frac{1}{\sqrt{2}}\Big(\cos\phi(J_x^{+1,0} - J_x^{-1,0}) \\ & - \sin\phi(J_y^{+1,0} + J_y^{-1,0})\Big) \\ & - \frac{1}{2}\left(\cos 2\phi J_x^{+1,-1} - \sin 2\phi J_y^{+1,-1}\right)\,, \end{aligned} \tag{23}$$

$$\begin{aligned} S_z^R(\phi) =& \frac{1}{\sqrt{2}} S_z - \cos\phi\left(J_x^{+1,0} + J_x^{-1,0}\right) \\ & + \sin\phi\left(J_y^{+1,0} - J_y^{-1,0}\right)\,, \end{aligned} \tag{24}$$

where $J_x^{j,k} = (a_j^\dagger a_k + a_j a_k^\dagger)/2$ and $J_y^{j,k} = (a_j^\dagger a_k - a_j a_k^\dagger)/2i$ are pseudo-spin operators. They are linked to the matrix elements (22) via $\rho_{j,k} = \langle J_x^{j,k} + iJ_y^{j,k}\rangle/N$. From a fit to the reduced population $n_0^R(\phi)$ and reduced spin $s_z^R(\phi)$, we can reconstruct $\rho^{(1)}$ (fig. 5).

## V. STATE RECONSTRUCTION

We present here the procedure used to reconstruct the density matrix of the collective spin state of the atoms at the end of the ramp, assuming that a single spatial mode is occupied. Our analysis makes use of about 1100 shots taken after various rotations. We extract three independent quantities from each shot, $S_z^R$, $n_0^R$ and the total atom number $N$. The superscript $R$ means that this value was measured after a spin rotation had been applied to the state. We have used two reconstruction procedures, the maximum likelihood (MaxLik) approach based on Bayesian inference and the maximum entropy (MaxEnt) approach based on Jayne's principle [12, 13]. The results reported in the main text follow from the MaxLik reconstruction.

### A. Basis for the reconstructed state

In the SMA, the state of the system can be written as $\rho = \bigoplus_N \rho^{(N)}$, where $\rho^{(N)}$ is the restriction to the subspace with $N$ atoms. Each $\rho^{(N)}$ can be decomposed in the basis of the collective spin states $|N, S, M\rangle$, where $S$ has the same parity as $N$ due to the exchange symmetry.

From the measurement $\langle \hat{\mathbf{S}}^2 \rangle \simeq 10$, we deduce that the total weight of the states with a spin larger than $S_{\max}$ is less than $10/S_{\max}^2$ (this is a very rough bound). In practice, we reconstructed the state of the system with $S_{\max} = 20$ (we have increased $S_{\max}$ to 40 and verified that the reconstructed state were essentially identical).

After projection on the $S \le S_{\max}$ subspaces, the state of the system can be written as $\rho = \bigoplus_N \rho^{(N, S \le S_{\max})}$. We further make the hypothesis that the all matrices $\rho^{(N, S\le S_{\max})}$ where $N$ has a given parity are identical. Lower $N$ are *a-priori* more favorable to reach lower $S$ states, but for small enough fluctuations of $N$ this effect should be negligible. This approximation is supported by the fact that no detectable correlations between $N$ and $n_0^R$ or $S_z^R$ appear in the data, an observation which is confirmed by numerical simulations of the adiabatic ramp performed for various initial atom numbers. Therefore, we write the state of the spin as

$$\rho = \rho_{\rm even}^{(N)} \oplus \rho_{\rm odd}^{(N+1)} . \tag{25}$$

In practice, we performed the reconstruction for various $N$ within $104 \pm 15$, and found very similar results (see Sec. V B).

### B. Maximum likelihood reconstruction

*a. Principle.* Let $\mathcal{P}\left(\rho|\{x_j\}\right)$ be the probability for the system to be in the state $\rho$ given our set of measurement outcomes $\{x_j\}$. Bayes theorem yields

$$\mathcal{P}\left(\rho|\{x_j\}\right) = \frac{\mathcal{P}\left(\{x_j\}|\rho\right)\mathcal{P}(\rho)}{\sum_{\rho'} \mathcal{P}\left(\{x_j\}|\rho'\right)\mathcal{P}(\rho')} , \tag{26}$$

where $\mathcal{P}(\rho)$ contains the *a-priori* information that we have on the state. In our case, we only assume that the spin state can be written as in Eq. (25). If $\rho$ is of the type given in Eq. (25), $\mathcal{P}(\rho) \propto 1$ is independent on $\rho$, otherwise $\mathcal{P}(\rho) = 0$. Thus, Eq. (26) can be rewritten as

$$\mathcal{P}\left(\rho|\{x_j\}\right) = \frac{\mathcal{P}\left(\{x_j\}|\rho\right)}{\sum_{\rho'} \mathcal{P}\left(\{x_j\}|\rho'\right)} , \tag{27}$$

where the sum is taken over all states of the form given by Eq. (25). The MaxLik state $\rho_{\rm ML}^{(N)}$ is defined as the argument maximizing the functional $\mathcal{P}\left(\rho|\{x_j\}\right)$. Given our imaging noise on the total atom number, we are not able to measure reliably the parity of $N$. For this reason, we reduce $\{x_j\}$ to the measurement of $n_{0,j}^R$ and $S_{z,j}^R$ on shots $j$. For the spin measurements, we take into account the imaging noise using Eq. (20), which gives the probability to measure $S_{z,j}^R$ for a given $\rho$.

*b. Algorithm.* The algorithm that we use to maximize the likelihood of Eq. (27) is described in [14]. It has been used to reconstruct the state of spinor BECs in [15, 16]. We initiate the algorithm on $\rho = \hat{1}/(S_{\max}+1)^2$, and stop it when the fidelity between the states obtained after two consecutive iterations is larger than $1 - 10^{-3}$. The subspaces with different spin parities are never mixed by the reconstruction algorithm, so that the state naturally remains of the form (25).

*c. Uncertainty.* To evaluate the uncertainty on the reconstructed density matrix $\rho_{\rm ML}^{(N)}$, we follow the protocol described in [14]. From $\rho_{\rm ML}^{(N)}$, we generate random sets of possible outcomes for our measurements (in practice, we simulate our experiment 100 times). For each simulated set of measurements, we perform the reconstruction and obtain the maximum likelihood density matrix $\rho_{\rm ML,sim}^{(N)}$. We compute the fidelity between $\rho_{\rm ML}^{(N)}$ and $\rho_{\rm ML,sim}^{(N)}$

$$\mathcal{F}(\rho_{\rm ML}^{(N)}, \rho_{\rm ML,sim}^{(N)}) = {\rm Tr}\left(\sqrt{\sqrt{\rho_{\rm ML}^{(N)}}\,\rho_{\rm ML,sim}^{(N)}\sqrt{\rho_{\rm ML}^{(N)}}}\right)^2 , \tag{28}$$

and find on average $\overline{\mathcal{F}}(\rho_{\rm ML}^{(N)}, \rho_{\rm ML,sim}^{(N)}) = 0.94$ indicating a faithful reconstruction. We provide in table II the expectation values of some observables of interest calculated using $\rho_{\rm ML}^{(N)}$, and compare them (when possible) to direct measurements.

We also performed the reconstruction with different $N'$ within the range $N = 104 \pm 15$. We found a fidelity $\mathcal{F}(\rho_{\rm ML}^{(N)}, \rho_{\rm ML}^{(N')})$ always larger than 0.99. This insensitivity of the reconstruction with respect to $N$ originates from the fact that in the $|N, S, M\rangle$ basis, the spin operator does not depend on $N$, contrary to $\hat{n}_0$. Thus, the precise value of $N$ only intervenes when we take into account the measurement of $\hat{n}_0$; however, it is the spin measurement that gives most information on the state.

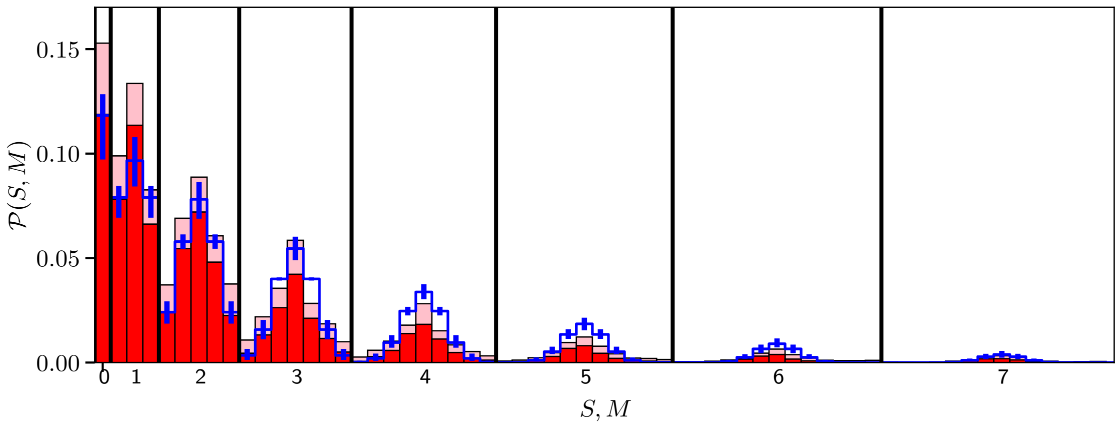


FIG. 6. Reconstructed MaxLik (red) and MaxEnt (blue) states in the $|S, M_z\rangle$ basis. Here, we show only the diagonal elements of the density matrices. The solid lines delimit the $S$ subspaces; within each subspace, the states are ordered by increasing $M_z$ from $-S$ to $+S$ (the labels refer to the value of $S$). The error bars (pink area for the MaxLik state) correspond to the 66% confidence interval.

| | $\langle \hat{n}_0 \rangle$ | $\langle \hat{\boldsymbol{S}}^2 \rangle$ | $\langle \hat{\Pi}_{S\leq 1} \rangle$ | $-\mathrm{Tr}(\rho \log \rho)$ |
|---|---|---|---|---|
| Direct meas. | $0.41 \pm 0.02$ | $9.9 \pm 0.1$ | - | - |
| $\rho_{\mathrm{ML}}^{(N)}$ | $0.40^{+0.01}_{-0.02}$ | $9.9^{+0.9}_{-0.2}$ | $0.44^{+0.13}_{-0.22}$ | $2.96^{+0.23}_{-0.07}$ |

TABLE II. Comparison between the predictions of the MaxLik reconstruction and direct measurements (when applicable). For $\langle \hat{n}_0 \rangle$, the error bar on the direct measurements corresponds to the statistical standard error. For $\langle \hat{\boldsymbol{S}}^2 \rangle$, the mean value and error bar are obtained for after deconvolution of the imaging noise (see § III). For the MaxLik state, we give the 68% confidence interval extracted from simulated data sets. The reconstruction is consistent with direct measurements of the one- and two-body observables $\langle \hat{n}_0 \rangle$ and $\langle \hat{\boldsymbol{S}}^2 \rangle$. However, it allows to go further and to infer the value of $N$-body observables, here $\hat{\Pi}_{S\leq 1}$, the projector onto the $S = 0$ and $S = 1$ spin manifolds. We can also compute non-linear functionals of the state $\rho_{\mathrm{ML}}^{(N)}$, such as the entropy.

### C. Maximum entropy reconstruction

*a. Principle.* In the MaxEnt approach, the expectation value $\overline{O}_i$ of an observable of interest $\hat{O}_i$ is extracted from the data set. The MaxEnt state $\rho_{\mathrm{ME}}$ is then defined as the state of maximal entropy, which verifies

$$\overline{O}_i = \mathrm{Tr}\left(\hat{O}_i \rho_{\mathrm{ME}}\right) . \tag{29}$$

Introducing Lagrange multipliers $\lambda_i$ to enforce the constraint (29), the MaxEnt state can be written as

$$\rho_{\mathrm{ME}} = \frac{1}{Z} \exp\left(-\sum_i \lambda_i \hat{O}_i\right) , \tag{30}$$

where $Z = \mathrm{Tr}\left(\exp\left(-\sum_i \lambda_i \hat{O}_i\right)\right)$ and the $\lambda_i$ are implicitly determined by the set of equations (29).

*b. Practical implementation.* We have chosen the set of observables $\{\hat{S}_z^2, \hat{S}_\perp^2, \hat{N}_{0z}, \hat{N}_{0x}\}$. From the measurements of the spin, we use the values given in table I obtained after noise removal, and we assume $S_x = S_y = S_\perp/2$. We do not use the data at intermediate rotations, because we do not have enough measurements for each angle to reliably extract an expectation value.

*c. Uncertainty.* We use the same methods as for the MaxLik approach and found $\overline{\mathcal{F}}(\rho_{\mathrm{ME}}^{(N)}, \rho_{\mathrm{ME,sim}}^{(N)}) \simeq 0.99$. Note that the uncertainties on the reconstruction have a different meaning in the MaxLik and MaxEnt approaches. Indeed, lack of information (*i.e.*, of measurements) results in an uncertainty for the MaxLik reconstruction and in a larger entropy for the MaxEnt state. For the latter, the uncertainty on the reconstruction only comes from imprecision on the measurements of the constraints $\langle O \rangle_i$.

### D. Results

The two reconstruction methods give very similar results. The fidelity between the two reconstructed states is $\mathcal{F}(\rho_{\mathrm{ML}}^{(N)}, \rho_{\mathrm{ME}}^{(N)}) \simeq 0.94$. We compare both reconstructions in figure 6. They are almost diagonal in the $|S, M_z\rangle$ basis and we thus only show the diagonal elements. The MaxEnt state has a slightly larger entropy, which was expected by construction. Note that part of the difference may be due to the smaller data set used for the reconstruction of $\rho_{\mathrm{ME}}$.

## VI. REDUCED DENSITY MATRIX

### A. General expression

The $n$-body reduced density matrix is defined as $\rho^{(n)} = \mathrm{Tr}_n^{(N)}(\rho)$, where $\mathrm{Tr}_n^{(N)}$ denotes the partial trace of the state of $N-n$ indistinguishable bosons among $N$ [17],

$$\mathrm{Tr}_n^{(N)}(\rho) = \frac{(N-n)!}{N!\,n!} \sum_{\substack{j_1..j_n\\ k_1..k_n}} \mathrm{Tr}^{(N)}(a_{j_1}^\dagger..a_{j_n}^\dagger a_{k_1}..a_{k_n}\rho) \times a_{j_1}^\dagger..a_{j_n}^\dagger a_{k_1}..a_{k_n} \qquad (31)$$

where the indices $j_l, k_l$ are summed over $0, \pm 1$, and $\mathrm{Tr}^{(N)}$ is the complete trace operation, *i.e.* over all $N$ particle states. After straightforward algebra, the matrix elements of $\rho^{(n)}$ in the $|N_{+1} = i_+, N_{-1} = i_-, N_0 = n - i_+ - i_-\rangle$ basis are shown to be

$$\left[\rho^{(n)}\right]_{i_+,i_-}^{j_+,j_-} = \binom{N}{n}^{-1} \langle \hat{P}^{(n)\dagger}_{i_+,i_-}\,\hat{P}^{(n)}_{j_+,j_-}\rangle\,, \qquad (32)$$

where

$$\hat{P}^{(n)}_{i_+,i_-} = \frac{\hat{a}_{+1}^{i_+}\;\hat{a}_{-1}^{i_-}\;\hat{a}_0^{n-i_+-i_-}}{\sqrt{i_+!\;i_-!\;(n-i_+-i_-)!}}\,. \qquad (33)$$

The $n$-body reduced density matrix has a clear physical meaning. It describes the state obtained after blindly removing $N-n$ atoms (*i.e.*, independently on their individual state). For the reconstructed state $\rho_{\mathrm{ML}}^{(N)}$, we compute $\rho_{\mathrm{ML}}^{(n)}$ numerically after projection on a state with fixed parity. The entropy and temperature shown in the main text are calculated for the reduced density matrices obtained after projection on the even parity sector. Projection on the odd parity sector yields essentially identical results.

### B. Singlet state

One can compute $\rho^{(n)}$ analytically for the $N$-particle singlet state. We start from the expression of the density matrix in the overcomplete basis formed by all polar states $|N:\mathbf{\Omega}\rangle = |m=0\rangle_{\mathbf{\Omega}}^{\otimes N}$ [5, 18, 19]

$$\rho_{\mathrm{s}}^{(N)} = \frac{N}{(4\pi)^2}\int d^2\mathbf{\Omega}\; d^2\mathbf{\Omega}'\;|N:\mathbf{\Omega}\rangle\langle N:\mathbf{\Omega}'|\,. \qquad (34)$$

This expression is convenient because the partial trace for coherent states takes the simple form

$$\mathrm{Tr}_n^{(N)}\left(|N:\mathbf{\Omega}\rangle\langle N:\mathbf{\Omega}'|\right) = |n:\mathbf{\Omega}\rangle\langle n:\mathbf{\Omega}'| \times \mathrm{Tr}^{(N-n)}\left(|N-n:\mathbf{\Omega}\rangle\langle N-n:\mathbf{\Omega}'|\right)\,.$$

The trace $\mathrm{Tr}^{(N-n)}$ can be calculated in the spin state basis using [19]

$$\langle N:\mathbf{\Omega}|NSM\rangle = \sqrt{f_S^N}\;Y_{SM}(\mathbf{\Omega})\,, \qquad (35)$$

where the $Y_{SM}$ are the spherical harmonics and [19]

$$f_S^N = \frac{4\pi\,2^S\;N!\;(\frac{N+S}{2})!}{(\frac{N-S}{2})!\;(N+S+1)!}\,. \qquad (36)$$

We obtain

$$\rho_{\mathrm{s}}^{(n)} = \frac{N}{(4\pi)^2}\sum_{SM} f_S^{N-n}\int d^2\mathbf{\Omega}\;Y_{SM}(\mathbf{\Omega})\;Y^*_{SM}(\mathbf{\Omega}')\;|n:\mathbf{\Omega}\rangle\langle n:\mathbf{\Omega}'|\,.$$

Using [19]

$$|nSM\rangle = \frac{1}{\sqrt{f_S^n}}\int d^2\mathbf{\Omega}\;Y_{SM}(\mathbf{\Omega})\;|n:\mathbf{\Omega}\rangle\,, \qquad (37)$$

we arrive at

$$\rho_{\mathrm{s}}^{(n)} = \frac{N}{(4\pi)^2}\sum_{SM} f_S^n\;f_S^{N-n}\;|nSM\rangle\langle nSM|\,. \qquad (38)$$

For $S \gg 1$ and $N \gg 1$, we have

$$f_S^N \simeq \frac{4\pi}{N}\mathrm{e}^{-\frac{S^2}{2N}}\,. \qquad (39)$$

Providing $n \gg 1$ and $N-n \gg 1$, we can use this approximation in $\rho_{\mathrm{s}}^{(n)}$ and we recognize the expression of a thermal state

$$\rho_{\mathrm{s}}^{(n)} \simeq \frac{1}{Z_n}\exp\left(-\frac{\hat{H}}{k_{\mathrm{B}}T_n}\right)\,, \qquad (40)$$

given the Hamiltonian $\hat{H} = \frac{U_s}{2N}\hat{\mathbf{S}}^2$ and the temperature

$$T_n = \frac{U_s}{k_{\mathrm{B}}}\frac{n}{N}\left(1-\frac{n}{N}\right)\,, \qquad (41)$$

with $k_{\mathrm{B}}$ the Boltzmann constant. The partition function is $Z_n = n(1-n/N)$. From this, the von Neumann entropy can be directly calculated, introducing $\beta_n = T_n^{-1}$:

$$\mathcal{S}_n \simeq \frac{d}{d\beta_n}\left(\beta_n \ln Z_n\right) \simeq \ln\left[n\left(1-\frac{n}{N}\right)\right] + 1\,. \qquad (42)$$

[1] Y. Kawaguchi and M. Ueda, "Spinor Bose–Einstein condensates," *Physics Reports*, vol. 520, pp. 253–381, Nov. 2012.

[2] C. K. Law, H. Pu, and N. P. Bigelow, "Quantum spin mixing in spinor Bose-Einstein condensates," *Phys. Rev. Lett.*, vol. 81, p. 5257, 1998.

[3] M. Koashi and M. Ueda, "Exact eigenstates and magnetic response of spin-1 and spin-2 Bose–Einstein condensates," *Physical Review Letters*, vol. 84, no. 6, p. 1066, 2000.

[4] Y. Castin and J. Dalibard, "Relative phase of two bose-einstein condensates," *Phys. Rev. A*, vol. 55, pp. 4330–4337, Jun 1997.

[5] S. Ashhab and A. J. Leggett, "Measurement theory and interference of spinor Bose-Einstein condensates," *Phys. Rev. A*, vol. 65, p. 023604, Jan 2002.

[6] J. Dalibard, Y. Castin, and K. Mølmer, "Wave-function approach to dissipative processes in quantum optics," *Phys. Rev. Lett.*, vol. 68, pp. 580–583, Feb 1992.

[7] H. Carmichael, *An open systems approach to quantum optics: lectures presented at the Université Libre de Bruxelles, October 28 to November 4, 1991*, vol. 18. Springer Science & Business Media, 2009.

[8] R. Dum, P. Zoller, and H. Ritsch, "Monte Carlo simulation of the atomic master equation for spontaneous emission," *Physical Review A*, vol. 45, no. 7, p. 4879, 1992.

[9] In principle, in this formalism one should also take into account a non-Hermitian contribution to the Hamiltonian. However, for the set of jump operators considered here, this non-Hermitian contribution is proportional to the total atom number and thus plays no role in the dynamics.

[10] D. Jaksch, C. W. Gardiner, K. M. Gheri, and P. Zoller, "Quantum kinetic theory. IV. Intensity and amplitude fluctuations of a Bose-Einstein condensate at finite temperature including trap loss," *Phys. Rev. A*, vol. 58, pp. 1450–1464, Aug 1998.

[11] A. Qu, B. Evrard, J. Dalibard, and F. Gerbier, "Probing entanglement in a spinor condensate near the single atom level," *arXiv 2004.09003*, 2020.

[12] G. M. D'Ariano, M. G. Paris, and M. F. Sacchi, "Quantum tomography," *Advances in Imaging and Electron Physics*, vol. 128, pp. 206–309, 2003.

[13] V. Bužek, R. Derka, G. Adam, and P. Knight, "Reconstruction of quantum states of spin systems: From quantum Bayesian inference to quantum tomography," *Annals of Physics*, vol. 266, no. 2, pp. 454–496, 1998.

[14] A. I. Lvovsky, "Iterative maximum-likelihood reconstruction in quantum homodyne tomography," *Journal of Optics B: Quantum and Semiclassical Optics*, vol. 6, pp. S556–S559, may 2004.

[15] J. Peise, I. Kruse, K. Lange, B. Lücke, L. Pezzè, J. Arlt, W. Ertmer, K. Hammerer, L. Santos, A. Smerzi, and C. Klempt, "Satisfying the Einstein–Podolsky–Rosen criterion with massive particles," *Nature Communications*, vol. 6, Nov. 2015.

[16] H. Strobel, W. Muessel, D. Linnemann, T. Zibold, D. B. Hume, L. Pezze, A. Smerzi, and M. K. Oberthaler, "Fisher information and entanglement of non-gaussian spin states," *Science*, vol. 345, pp. 424–427, July 2014.

[17] M. Gessner and A. Buchleitner, "On the reduced dynamics of a subset of interacting bosonic particles," *Annals of Physics*, vol. 390, pp. 192–213, Mar. 2018.

[18] Y. Castin and C. Herzog, "Bose–Einstein condensates in symmetry breaking states," *Comptes Rendus de l'Académie des Sciences - Series IV - Physics*, vol. 2, no. 3, pp. 419 – 443, 2001.

[19] R. Barnett, J. D. Sau, and S. Das Sarma, "Antiferromagnetic spinor condensates are quantum rotors," *Phys. Rev. A*, vol. 82, p. 031602, Sep 2010.
